# Supplementary material for: How the world's collective attention is being paid to a pandemic: COVID-19 related n-gram time series for 24 languages on Twitter
Source: arXiv:2003.12614 source file (2021-01-06)
Supplement: Supplementary file 1 [file covid19-ngrams.appendix.tex]

%\begin{table*}[h]
%  \centering
%  \begin{tabular}{l|l|l}
%    \textbf{Country} & \textbf{Language} & \textbf{List of selected $1$-grams} \\
%    \hline
%    United States & {English} (en) &  {`virus', `coronavirus', `COVID-19', `pandemic', `\#COVID19'} \\
%    Mexico & {Spanish}    (es) &  {`virus', `coronavirus', `cuarentena', `pandemia', `\#COVID19'} \\
%    Brazil & {Portuguese} (pt) &  {`vírus', `corona', `quarentena', `coronavírus', `\#COVID19'} \\
%    %Saudi Arabia & {Arabic}     (ar) & {`فيروس', `كورونا', `الوباء', `#فيروس_كورونا', `\#كورونا'} \\
%    France & {French}     (fr) & {`virus', `quarantaine', `confinement', `Coronavirus', `\#COVID19'} \\
%    Indonesia & {Indonesian} (id) & {`virus', `corona', `pandemi', `masker', `\#COVID19'} \\
%    Turkey & {Turkish}    (tr) & {`virüs', `Koronavirüs', `maske', `korona', `\#COVID19'} \\
%    Germany & {German}     (de) & {`Virus', `Corona', `Coronavirus', `Quarantäne', `\#COVID19'} \\
%    Italy & {Italian}    (it) & {`virus', `quarantena', `Coronavirus', `pandemia', `\#COVID19'} \\
%    Russia & {Russian}    (ru) & {`вирус', `карантин', `коронавируса', `самоизоляции', `\#COVID19'} \\
%    India & {Hindi}      (hi) & {`virus', `मरकज', `तबल', `\#lockdown', `\#COVID19'} \\
%    %Iran & {Persian}    (fa) & {`ویروس', `قرنطینه', `کرونا', `\#كرونا', `\#کروناویروس'} \\
%  \end{tabular}
%  \caption{
%    ..
%  }
%  \label{tab:covid19.coronagrams_cases}
%\end{table*}


\begin{figure*}[tp!] 
  \includegraphics[width=\textwidth]{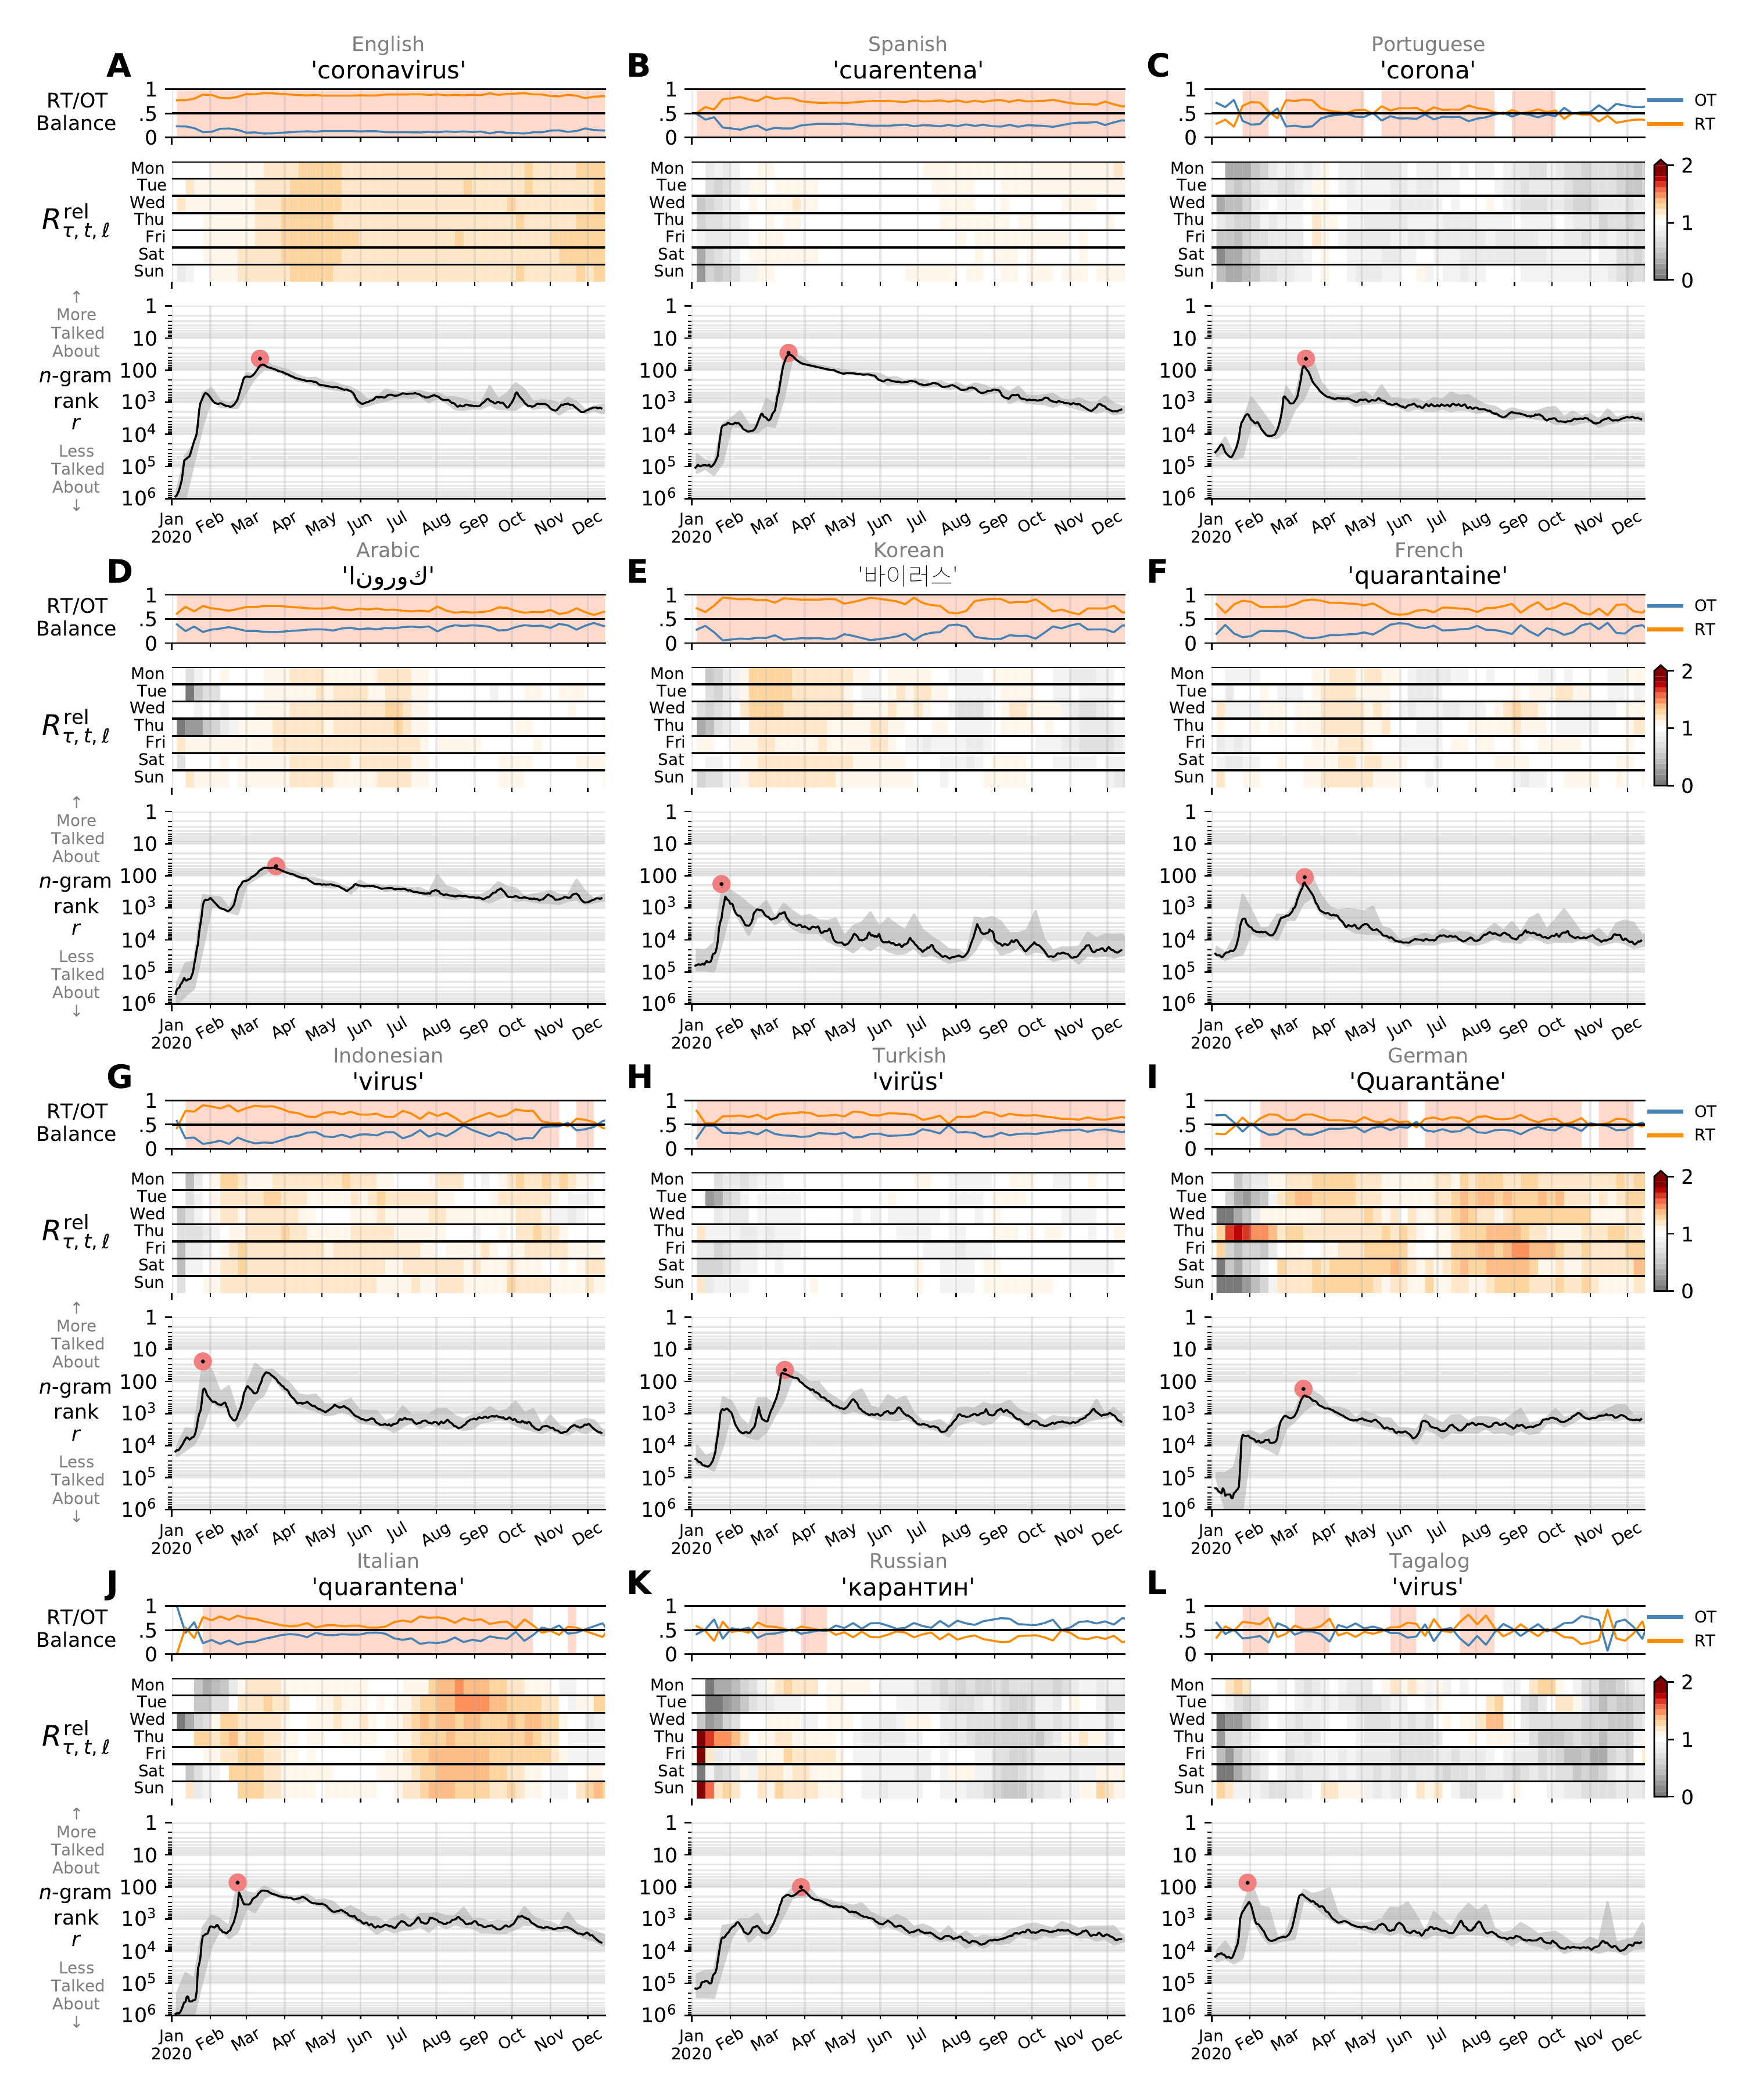}
  \caption{
    A collection of salient 1-grams across the top 12 languages for April 2020 relative to April 2019.
  }
  \label{fig:covid19.1grams_samples}
\end{figure*}


\begin{figure*}[tp!]
  \includegraphics[width=\textwidth]{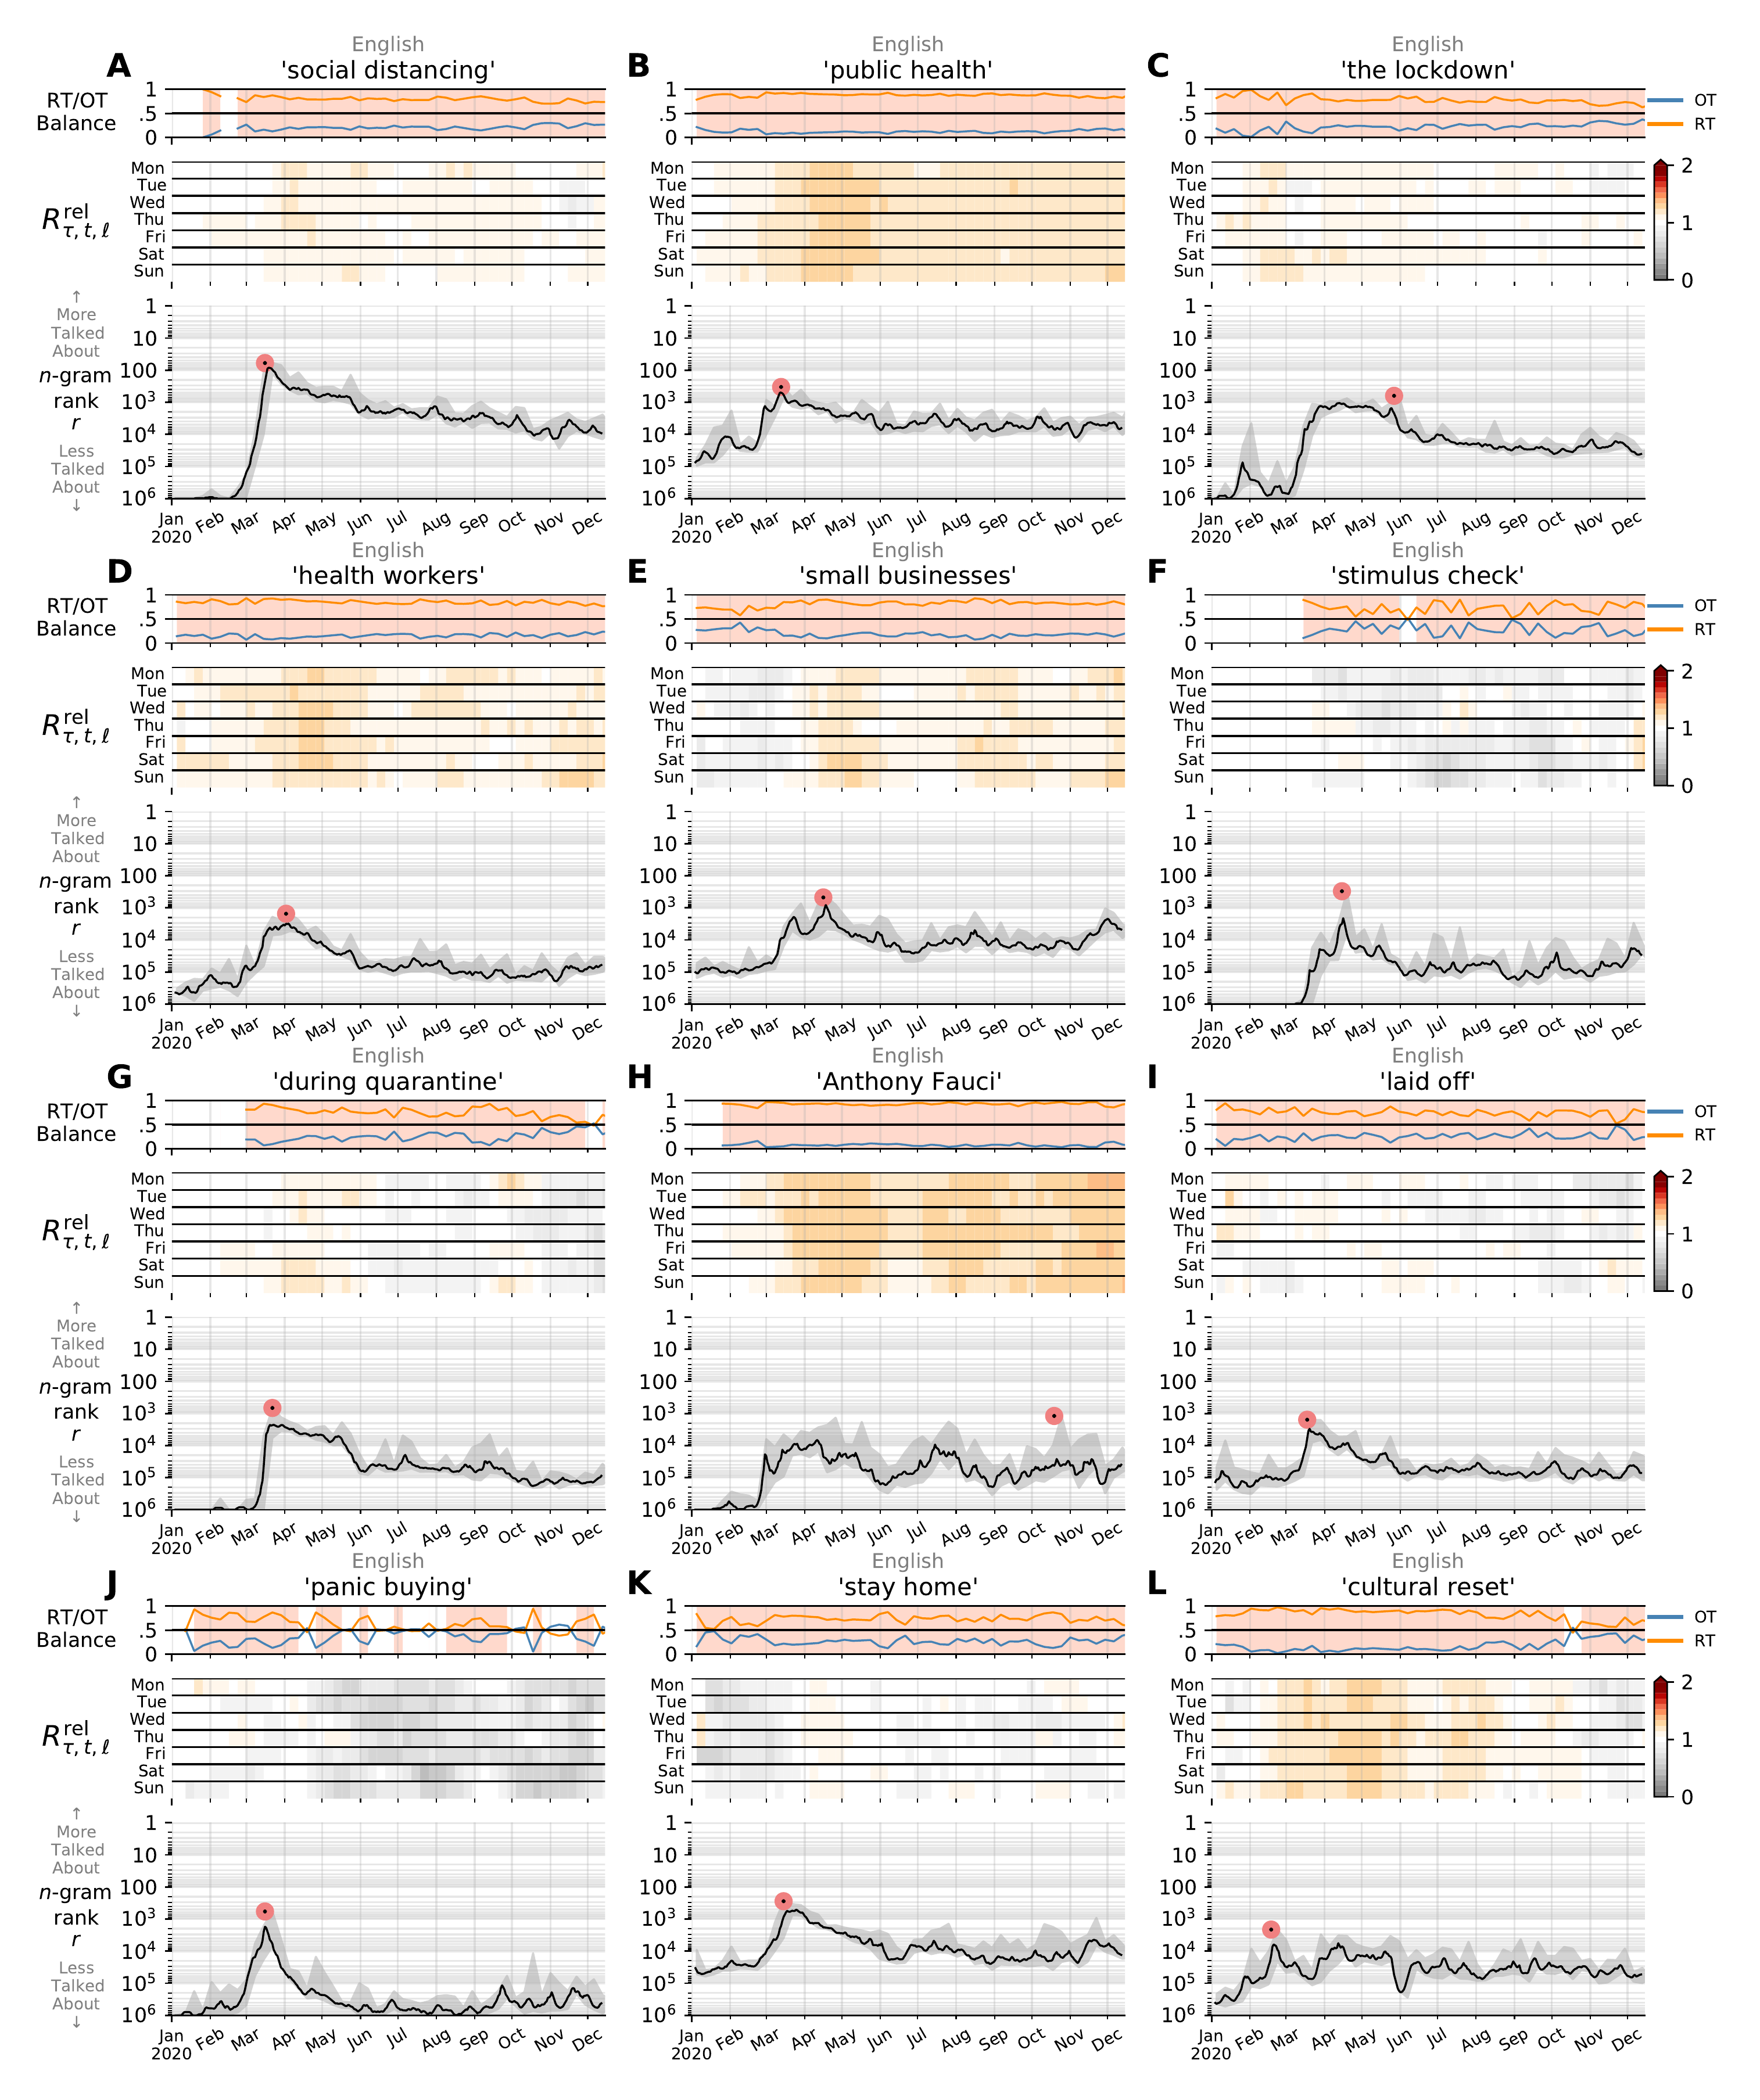}
  \caption{
    A collection of salient English 2-grams for April 2020 relative to April 2019.
    We note a rich and wide range of cultural, geopolitical and socioeconomic references in the selected 2-grams. 
  }
  \label{fig:covid19.2grams_samples}
\end{figure*}
